# Supplementary material for: Teaching Concurrent Software Design: A Case Study Using Android
Source: arXiv:1705.02899 source file (2017-05-08)
Supplement: Supplementary file 1 [file appendix.tex]

\addcontentsline{toc}{chapter}{APPENDICES}

%%%%%%%%%%CHANGE HERE%%%%%%%%%%
