# Supplementary material for: Teaching Concurrent Software Design: A Case Study Using Android
Source: arXiv:1705.02899 source file (2017-05-08)
Supplement: Supplementary file 2 [file appendixa.tex]

%\chapter*{}
%\Section{TEXT WATERMARKING TABLES}\label{chap:textwatermarkingtables}
\chapter {GIS Data Sizes}\label{chap:textwatermarkingtables}
%\Section{TEXT WATERMARKING TABLES}\label{chap:textwatermarkingtables}
%\addcontentsline{toc}{section}{APPENDIX A: \hspace{.2in}TEXT WATERMARKING TABLES}
%\chaptermark{Appendix}
%\markboth{Appendix}{Appendix}
%\section{Text Watermarking Results}

%%Table Example

%If you have a lot of tables like I did you will need the clearpage to prevent too many unprocessed floats errors
\clearpage
% \vspace{0.4in}
%\clearpage
%\newpage
