# Supplementary material for: Teaching Concurrent Software Design: A Case Study Using Android
Source: arXiv:1705.02899 source file (2017-05-08)
Supplement: Supplementary file 3 [file appendixb.tex]

\chapter[WATERMARKING TABLES]{WATERMARKING TABLES}\label{chap:happyfacewatermarkingtables}

Appendix B goes here

\clearpage
